# Supplementary material for: Real Time Trajectory Prediction Using Deep Conditional Generative Models
Source: arXiv:1909.03895 source file (2020-01-07)
Supplement: Supplementary file 1 [file supplementary.pdf]

# Real Time Trajectory Prediction Using Deep Conditional Generative Models: Supplementary Material

*Sebastian Gomez-Gonzalez, Sergey Prokudin, Bernhard Schölkopf and Jan Peters*

## 1 Derivation of the Lower Bound on the Conditional Log Likelihood

The probability distribution over the latent variable $\boldsymbol{z}$ given an entire trajectory $\boldsymbol{y}_{1:T}$ can be expressed using Bayes rule with the generative distributions presented in the paper, obtaining

$$p(\boldsymbol{z} \mid \boldsymbol{y}_{1:T}) = p(\boldsymbol{z} \mid \boldsymbol{y}_{1:t-1}, \boldsymbol{y}_{t:T}) = \frac{p(\boldsymbol{y}_{t:T} \mid \boldsymbol{y}_{1:t-1}, \boldsymbol{z}) p(\boldsymbol{z} \mid \boldsymbol{y}_{1:t-1})}{p(\boldsymbol{y}_{t:T} \mid \boldsymbol{y}_{1:t-1})},$$

where $p(\boldsymbol{y}_{t:T} \mid \boldsymbol{y}_{1:t-1})$ is the conditional likelihood, whose computation requires evaluating an intractable integral over $\boldsymbol{z}$, and is given by

$$p(\boldsymbol{y}_{t:T} \mid \boldsymbol{y}_{1:t-1}) = \int p(\boldsymbol{y}_{t:T} \mid \boldsymbol{y}_{1:t-1}, \boldsymbol{z}) p(\boldsymbol{z} \mid \boldsymbol{y}_{1:t-1}) d\boldsymbol{z}.$$

If we use a variational distribution $q(\boldsymbol{z}|\boldsymbol{y}_{1:T})$ to approximate the intractable distribution $p(\boldsymbol{z} \mid \boldsymbol{y}_{1:T})$, we can write the log conditional likelihood as

$$\log p(\boldsymbol{y}_{t:T} \mid \boldsymbol{y}_{1:t-1}) = -\operatorname{KL}(q(\boldsymbol{z} \mid \boldsymbol{y}_{1:T}) \| p(\boldsymbol{z} \mid \boldsymbol{y}_{1:T})) + \mathbb{E}_{q(\boldsymbol{z} \mid \boldsymbol{y}_{1:T})}[\log p(\boldsymbol{y}_{t:T}, \boldsymbol{z} \mid \boldsymbol{y}_{1:t-1}) - \log q(\boldsymbol{z} \mid \boldsymbol{y}_{1:T})].$$

The previous equation can be easily verified by expanding the KL divergence and the expectation integrals on the right hand side on the equation, and applying simple logarithm properties and expanding the probability distributions with the equations provided in this section until the left hand of the equation is obtained. Now, we proceed to construct a lower bound on $\log p(\boldsymbol{y}_{t:T} \mid \boldsymbol{y}_{1:t-1})$ from the previous equation using the fact that the KL divergence is a non-negative number. Subsequently, we use standard rules of probability to transform the lower bound to the one used on the paper, obtaining

$$\begin{aligned}
\log p(\boldsymbol{y}_{t:T} \mid \boldsymbol{y}_{1:t-1}) &\geq \mathbb{E}_{q(\boldsymbol{z} \mid \boldsymbol{y}_{1:T})}[\log p(\boldsymbol{y}_{t:T}, \boldsymbol{z} \mid \boldsymbol{y}_{1:t-1}) - \log q(\boldsymbol{z} \mid \boldsymbol{y}_{1:T})] \\
&= \mathbb{E}_{q(\boldsymbol{z} \mid \boldsymbol{y}_{1:T})}[\log p(\boldsymbol{z} \mid \boldsymbol{y}_{1:t-1}) + \log p(\boldsymbol{y}_{t:T} \mid \boldsymbol{z}, \boldsymbol{y}_{1:t-1}) - \log q(\boldsymbol{z} \mid \boldsymbol{y}_{1:T})] \\
&= \mathbb{E}_{q(\boldsymbol{z} \mid \boldsymbol{y}_{1:T})}[-\log q(\boldsymbol{z} \mid \boldsymbol{y}_{1:T}) + \log p(\boldsymbol{z} \mid \boldsymbol{y}_{1:t-1})] + \mathbb{E}_{q(\boldsymbol{z} \mid \boldsymbol{y}_{1:T})}[\log p(\boldsymbol{y}_{t:T} \mid \boldsymbol{z}, \boldsymbol{y}_{1:t-1})] \\
&= \operatorname{KL}(q(\boldsymbol{z} \mid \boldsymbol{y}_{1:T}) \| p(\boldsymbol{z} \mid \boldsymbol{y}_{1:t-1})) + \mathbb{E}_{q(\boldsymbol{z} \mid \boldsymbol{y}_{1:T})}[\log p(\boldsymbol{y}_{t:T} \mid \boldsymbol{y}_{1:t-1}, \boldsymbol{z})].
\end{aligned}$$

Note that both $q(\boldsymbol{z} \mid \boldsymbol{y}_{1:T})$ and $p(\boldsymbol{z} \mid \boldsymbol{y}_{1:t-1})$ are distributions that map from observation space to the latent space, acting both as encoders, one for full trajectories and the other for partial trajectories. Using the masked variables $\boldsymbol{x}^t$ and $\hat{\boldsymbol{x}}^t$ we can use a single encoder network $\boldsymbol{g}_\phi$ to encode both partial and full trajectories. We can write the lower bound as

$$\log p_\theta(\boldsymbol{y}_{t:T} \mid \boldsymbol{y}_{1:t-1}) \geq -\operatorname{KL}(q_\phi(\boldsymbol{z} \mid \boldsymbol{y}_{1:T}) \| q_\phi(\boldsymbol{z} \mid \boldsymbol{y}_{1:t-1})) + \mathbb{E}_{q_\phi(\boldsymbol{z} \mid \boldsymbol{y}_{1:T})}[\log p(\boldsymbol{y}_{t:T} \mid \boldsymbol{y}_{1:t-1}, \boldsymbol{z})],$$

arriving to the resulting lower bound presented on the paper. This lower bound is optimized to find the parameters of the encoder $\boldsymbol{\phi}$ and decoder $\boldsymbol{\theta}$ networks, as well as distribution parameters such as $\boldsymbol{\Sigma}_y$.

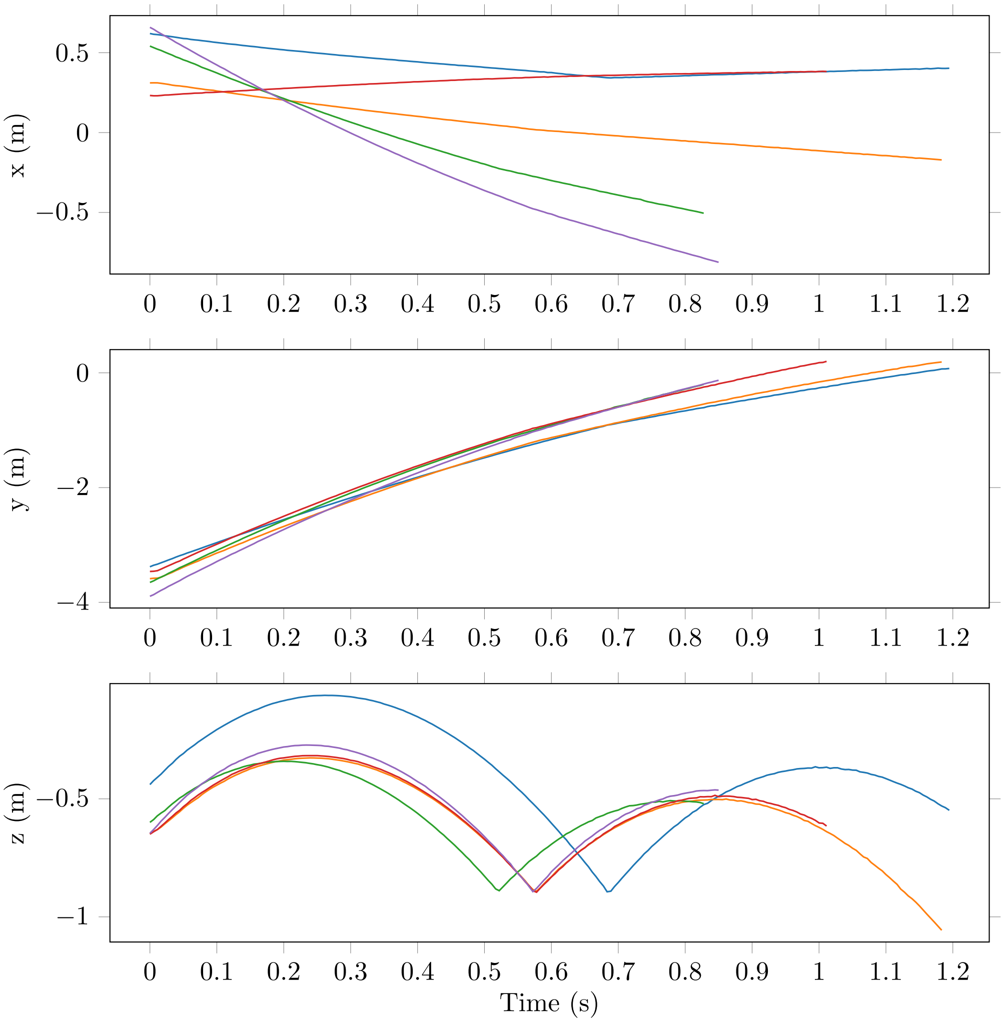


Fig. 1: Different samples of table tennis ball trajectories in X, Y and Z (in meters) with respect to time (in seconds). The five ball trajectories depicted in this figure where taken randomly from the ball trajectory dataset collected with the robot vision system.

## 2 Ball Trajectory Experiments

For the ball trajectory experiments we used a vision system proposed in previous work to collect the ground truth data. As mentioned on the paper, we do not have access to the spin information, only 3D positions. Figure 1 shows 5 random trajectories from the training set collected on the real system. Notice that there is little variability in the $Y$ coordinate, since the ball is always coming from the opponent's court towards the robot. The opponent typically hits the ball anywhere between $Y = 3.5$ to $Y = 4$, and the ball subsequently fly towards the robot whose center is located exactly at $Y = 0$. In the other coordinates there is more variability. The trajectory durations vary typically between 0.8 and 1.2 seconds.

We decided to include the data sets we used for training and validation in the supplementary material as well to allow for more easy comparison in the future. The files are called "ball_traj_train.npz" and "ball_traj_test.npz" for the training and validation set respectively. We also included a Python script to plot trajectories from the training or validation sets. The latency of the training procedure is not reported in the paper because it does not need to run in real time. For completeness, we report here a running time of 12m:52s for the training procedure using 200 training epochs in the same computer were the other experiments were reported.
